# Supplementary material for: Exploring the Geometry and Topology of Neural Network Loss Landscapes
Source: arXiv:2102.00485 source file (2022-01-26)
Supplement: Supplementary file 1 [file appendix.tex]

\vspace{-5pt}
\section{Related work}\label{s:related_work}
\vspace{-7pt}
\subsection{Loss landscape visualization}\label{ss:ll_visualization}
Loss landscape visualization methods have been proposed in numerous contexts. \citet{goodfellow2014qualitatively} proposed the ``linear path experiment'' where the loss of an ANN is evaluated at a series of points $\theta=(1-\alpha)\theta_i + \alpha \theta_f$ for different values of $\alpha \in [0,1]$ and $\theta_i,\theta_f$ corresponding to the initial parameters of the model and the found optima in parameter space respectively. This one-dimensional linear interpolation method has allowed them to show that popular state of the art ANNs typically do not encounter significant obstacles along a straight path from initialization to convergent solution. They also used the method to visualize the loss along directions connecting two distinct minima and to show that these are linearly separated by a region of higher valued loss.

This method was further developed by \citet{im2016empirical_loss_surfaces}, who adapted it to enable the visualization of two-dimensional projections of the loss-landscape using barycentric and bilinear interpolation for groups of three or four points in parameter space. This analysis method has allowed them to establish that despite starting with the same parameter initialization, different optimization algorithms find different minima. Furthermore, they noticed that the loss-landscape around minima have characteristic shapes that are optimizer-specific and that batch-normalization smoothens the loss function.

More recently, \citet{Goldstein_LL_NIPS2018_7875} have addressed the \textit{scale invariance} and \textit{network symmetries} problems discussed in \citet{neyshabur2017exploring} and \citet{dinh2017sharp_minima_gen}, which prevented meaningful comparisons between loss-landscape plots from different networks. They proposed 1D and 2D linear interpolation plots, similar to past techniques, but where they used filter-wise normalized directions to remove the scaling effect. This method has allowed them to visualize and compare the regions on the loss-landscape surrounding minima coming from multiple networks in a meaningful way and to correlate the ``flatness'' of the region to the generalization capabilities of the corresponding network. Furthermore, they studied the effects of the network depth, width and the presence of skip connections on the geometry of the loss-landscape and on network generalization. %They also proposed using normalized PCA directions to plot training trajectories in two dimensions.

\subsection{Generalization and importance of studying the loss landscape}
Ensuring that machine learning models can generalize to new data is one of the most important steps in solving any data analysis task, and is a core problem in the field. The idea that a network's ability to generalize is linked to the geometry of the loss landscape around the optima was initially presented in \citet{Hochreiter1997_flat_minima} and has recently been the focus of numerous papers~\citep[e.g.,][]{entropy_sgd,keskar2016large_batch,swirszcz2016local_minima,dinh2017sharp_minima_gen,Goldstein_LL_NIPS2018_7875}. Flat minima in parameter space, around which the value of the loss function is fairly constant, are believed to correspond to configurations where the network generalizes well to the unseen data. Sharp minima, on the other hand, correspond to ones where the network is expected to generalize poorly. Following the underlying idea of these propositions, we believe that studying the geometry of the loss landscape around minima has the potential of uncovering key characteristics about the network's ability to generalize. 

Furthermore, the importance of loss landscape visualization methods like the one presented in this paper increases with the growing scientific community interest in furthering our understanding of ANNs. As our understanding of this landscape gets deeper, we start uncovering more and more high-dimensional and complex geometric and topological characteristics. For instance, \citet{essentially_no_barriers} have found nonlinear pathways in parameter space connecting distinct minima, along which the training and test errors remain small and losses are consistently low. This suggests that minima are not situated in isolated valleys but rather on connected manifolds representing low loss regions. However, such characteristics are intrinsically high-dimensional, making linear methods inadequate to visualize these structures. Even in standard applications of the linear methods one inevitably asks if the thousands (or even millions) of unseen directions do not hide critical features of the landscape, and if the visualized linear path is relevant to what happened during training.

\subsection{Manifold learning and topological data analysis}
In this paper, we suggest the use of modern manifold learning and topological data analysis techniques to study the complex loss landscape of ANNs. Manifold learning techniques have been extensively used in recent years to successfully study the internal learned representations of deep networks and highlight their complex geometric structures and intrinsic dimensionality \citep{gigante2019visualizing, horoi2020internal, recanatesi2018signatures, farrell2019dynamic, maheswaranathan2019universality}. Here we further advance theses lines of work to provide new applications and insights in the study of ANN optimization and generalization.

To our knowledge, this is the first time topological data analysis (TDA) has been applied to the study of ANN loss landscapes. 
However, the application of algebraic topology to the analysis of real-valued functions defined on manifolds is not novel, and is in fact at the heart of Morse theory, developed by Marston Morse and others during the 20$^{\text{th}}$ century~\citep{morse1925relations, milnor2016morse}. 
More recently, numerous efficient computational algorithms for solving concrete problems related to algebraic topology have been developed in the field of computational topology \citep{Edelsbrunner10}.
A particular problem that can be solved through the use of TDA algorithms is the topological characterization of critical points of real-valued functions defined on manifolds \citep{Gyulassy08, Gyulassy2006topological, bremer2004topological}. If the ambient dimension of the manifold is low~(2D or 3D), such a characterization gives rise to a decomposition of a function in terms of regions of similar gradient behavior~(the classical example is a function with two peaks defined on $\mathbf{R}^2$; here, there would be a decomposition into regions that measure which peak is ``closer''). This decomposition is known as the Morse--Smale complex. 
The Morse--Smale complex can be computed from the critical points of the respective function and its unstable manifolds as defined by the dynamics of gradient descent~(or ascent). 
The hierarchical structure of the complexes and the function's topological features are found by considering the succession of critical points and unstable manifolds in the increasing sequence of the function's sublevel sets, i.e., the set of all points on the manifold whose function value is less than or equal to a pre-defined threshold. 
The difference between the function values of different critical points---equivalently, this is the difference between the ``appearance'' and ``disappearance'' of a topological feautre---is referred to as the \emph{persistence}. Persistence  can be used to simplify a given function by smoothing out features; this is typically achieved by cancelling related pairs of critical points whose persistence fails to satisfy a certain simplification threshold.
Such analysis methods have been successfully applied in the field of electrochemistry, for instance, to characterize the topology of energy landscapes of different molecules \citep{Gyulassy2006topological, bremer2004topological}. 
This directly relates to our work since the loss-landscape associates a loss value to each point in the parameter space of the ANN and we wish to characterize the topology of this landscape. The primary difference to existing work is that we are dealing with a manifold whose~(ambient) dimension is much higher, thus precluding the analytical calculation of the Morse--Smale complex.

\clearpage
\section{}\label{a:dim_red_comparison_hi_res}
\begin{figure}[H]
    \centering
    \includegraphics[width=0.95\textwidth]{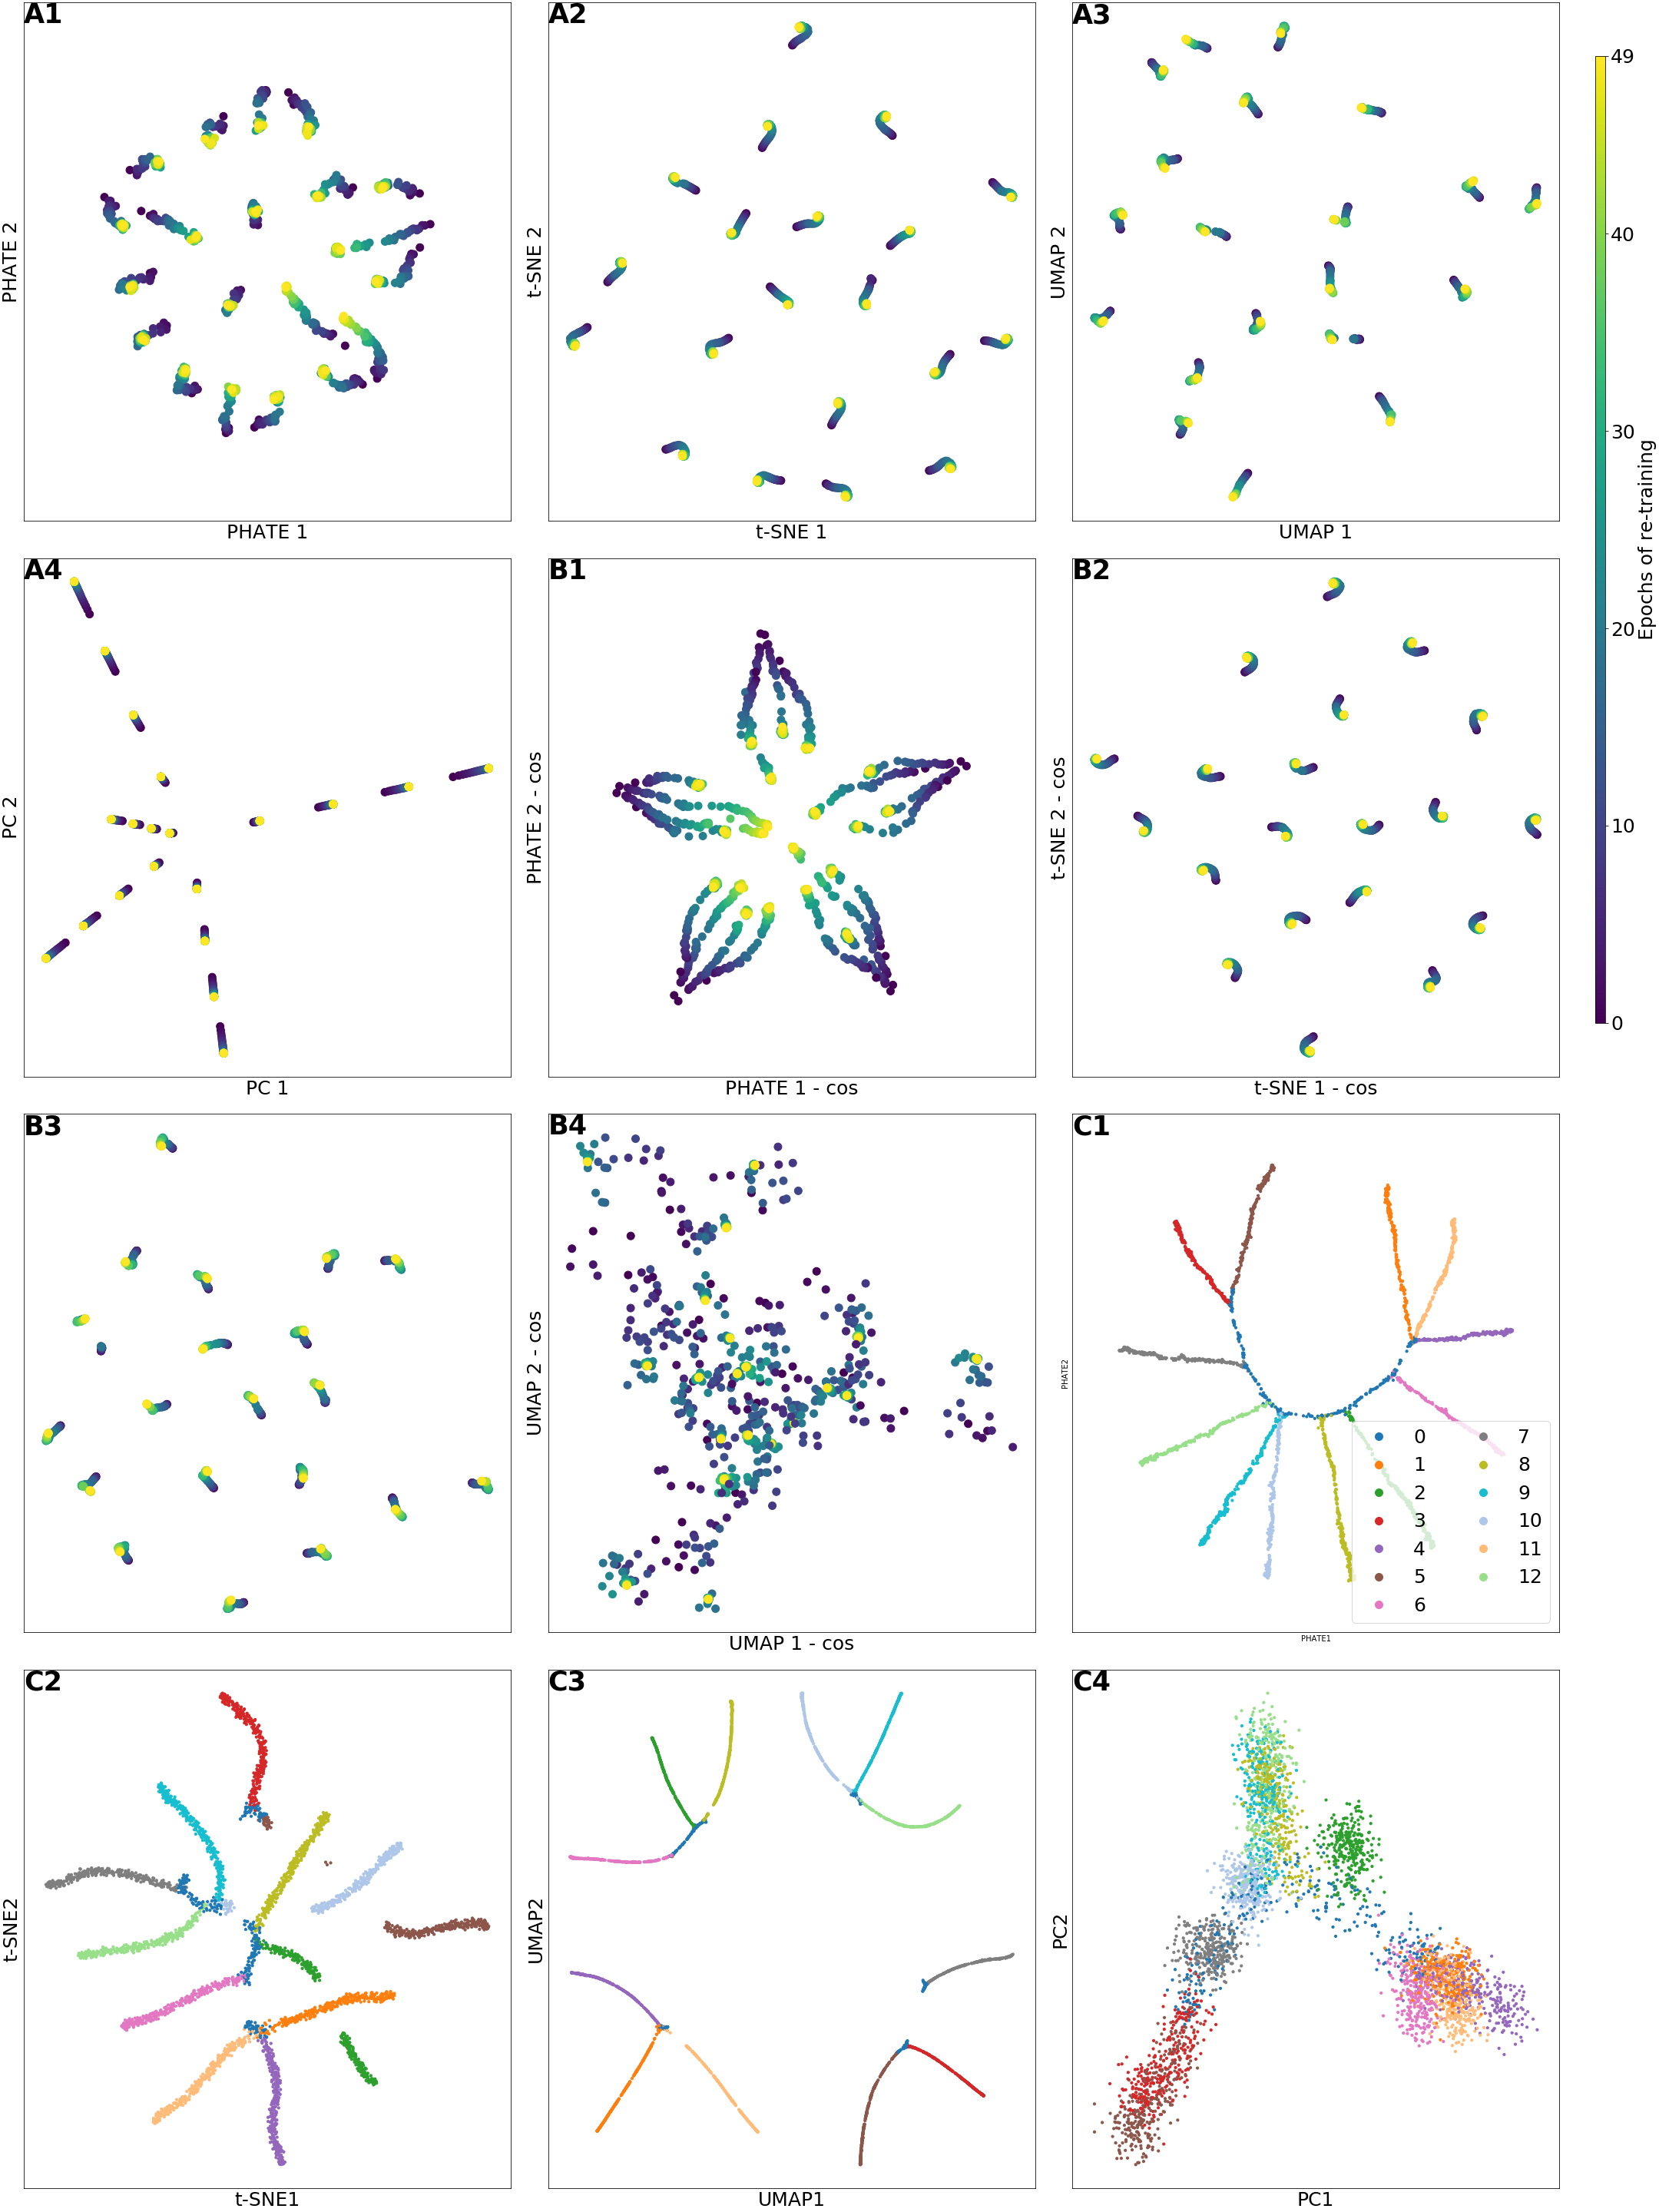}
    \caption{Higher resolutionversion of Figure \ref{fig:dim_red_comparison}}
    \label{fig:dim_red_comparison_hi_res}
\end{figure}

% \section{}\label{a:generalization_hi_res}
% \begin{figure}[H]
%     \centering
%     \includegraphics[width=0.95\textwidth]{figures/generalization_memorization_figure_appendix.png}
%     \caption{Higher resolution version of Figure \ref{fig:generalization}}
%     \label{fig:generalization_hi_res}
% \end{figure}

\clearpage
\section{}\label{a:classifiers}
The 11 classifiers were: k-NN classifier with k=5, linear SVM, RBF kernel SVM, Gaussian Process classifier, decision tree, random forest with 100 trees, MLP classifier with 1 hidden layer of 100 ReLU neurons trained with ADAM, AdaBoost classifier with base classifier a decision tree with depth 1, Gaussian Naive Bayes, Multinomial Naive Bayes and a Quadratic Discriminant Analysis classifier. The classifiers were trained and evaluated using 10-fold cross validation. The Scikit-learn implementations were used for all of them.

\clearpage
\section{}\label{a:robustness_hi_res}
\begin{figure}[H]
    \centering
    \includegraphics[width=0.95\textwidth]{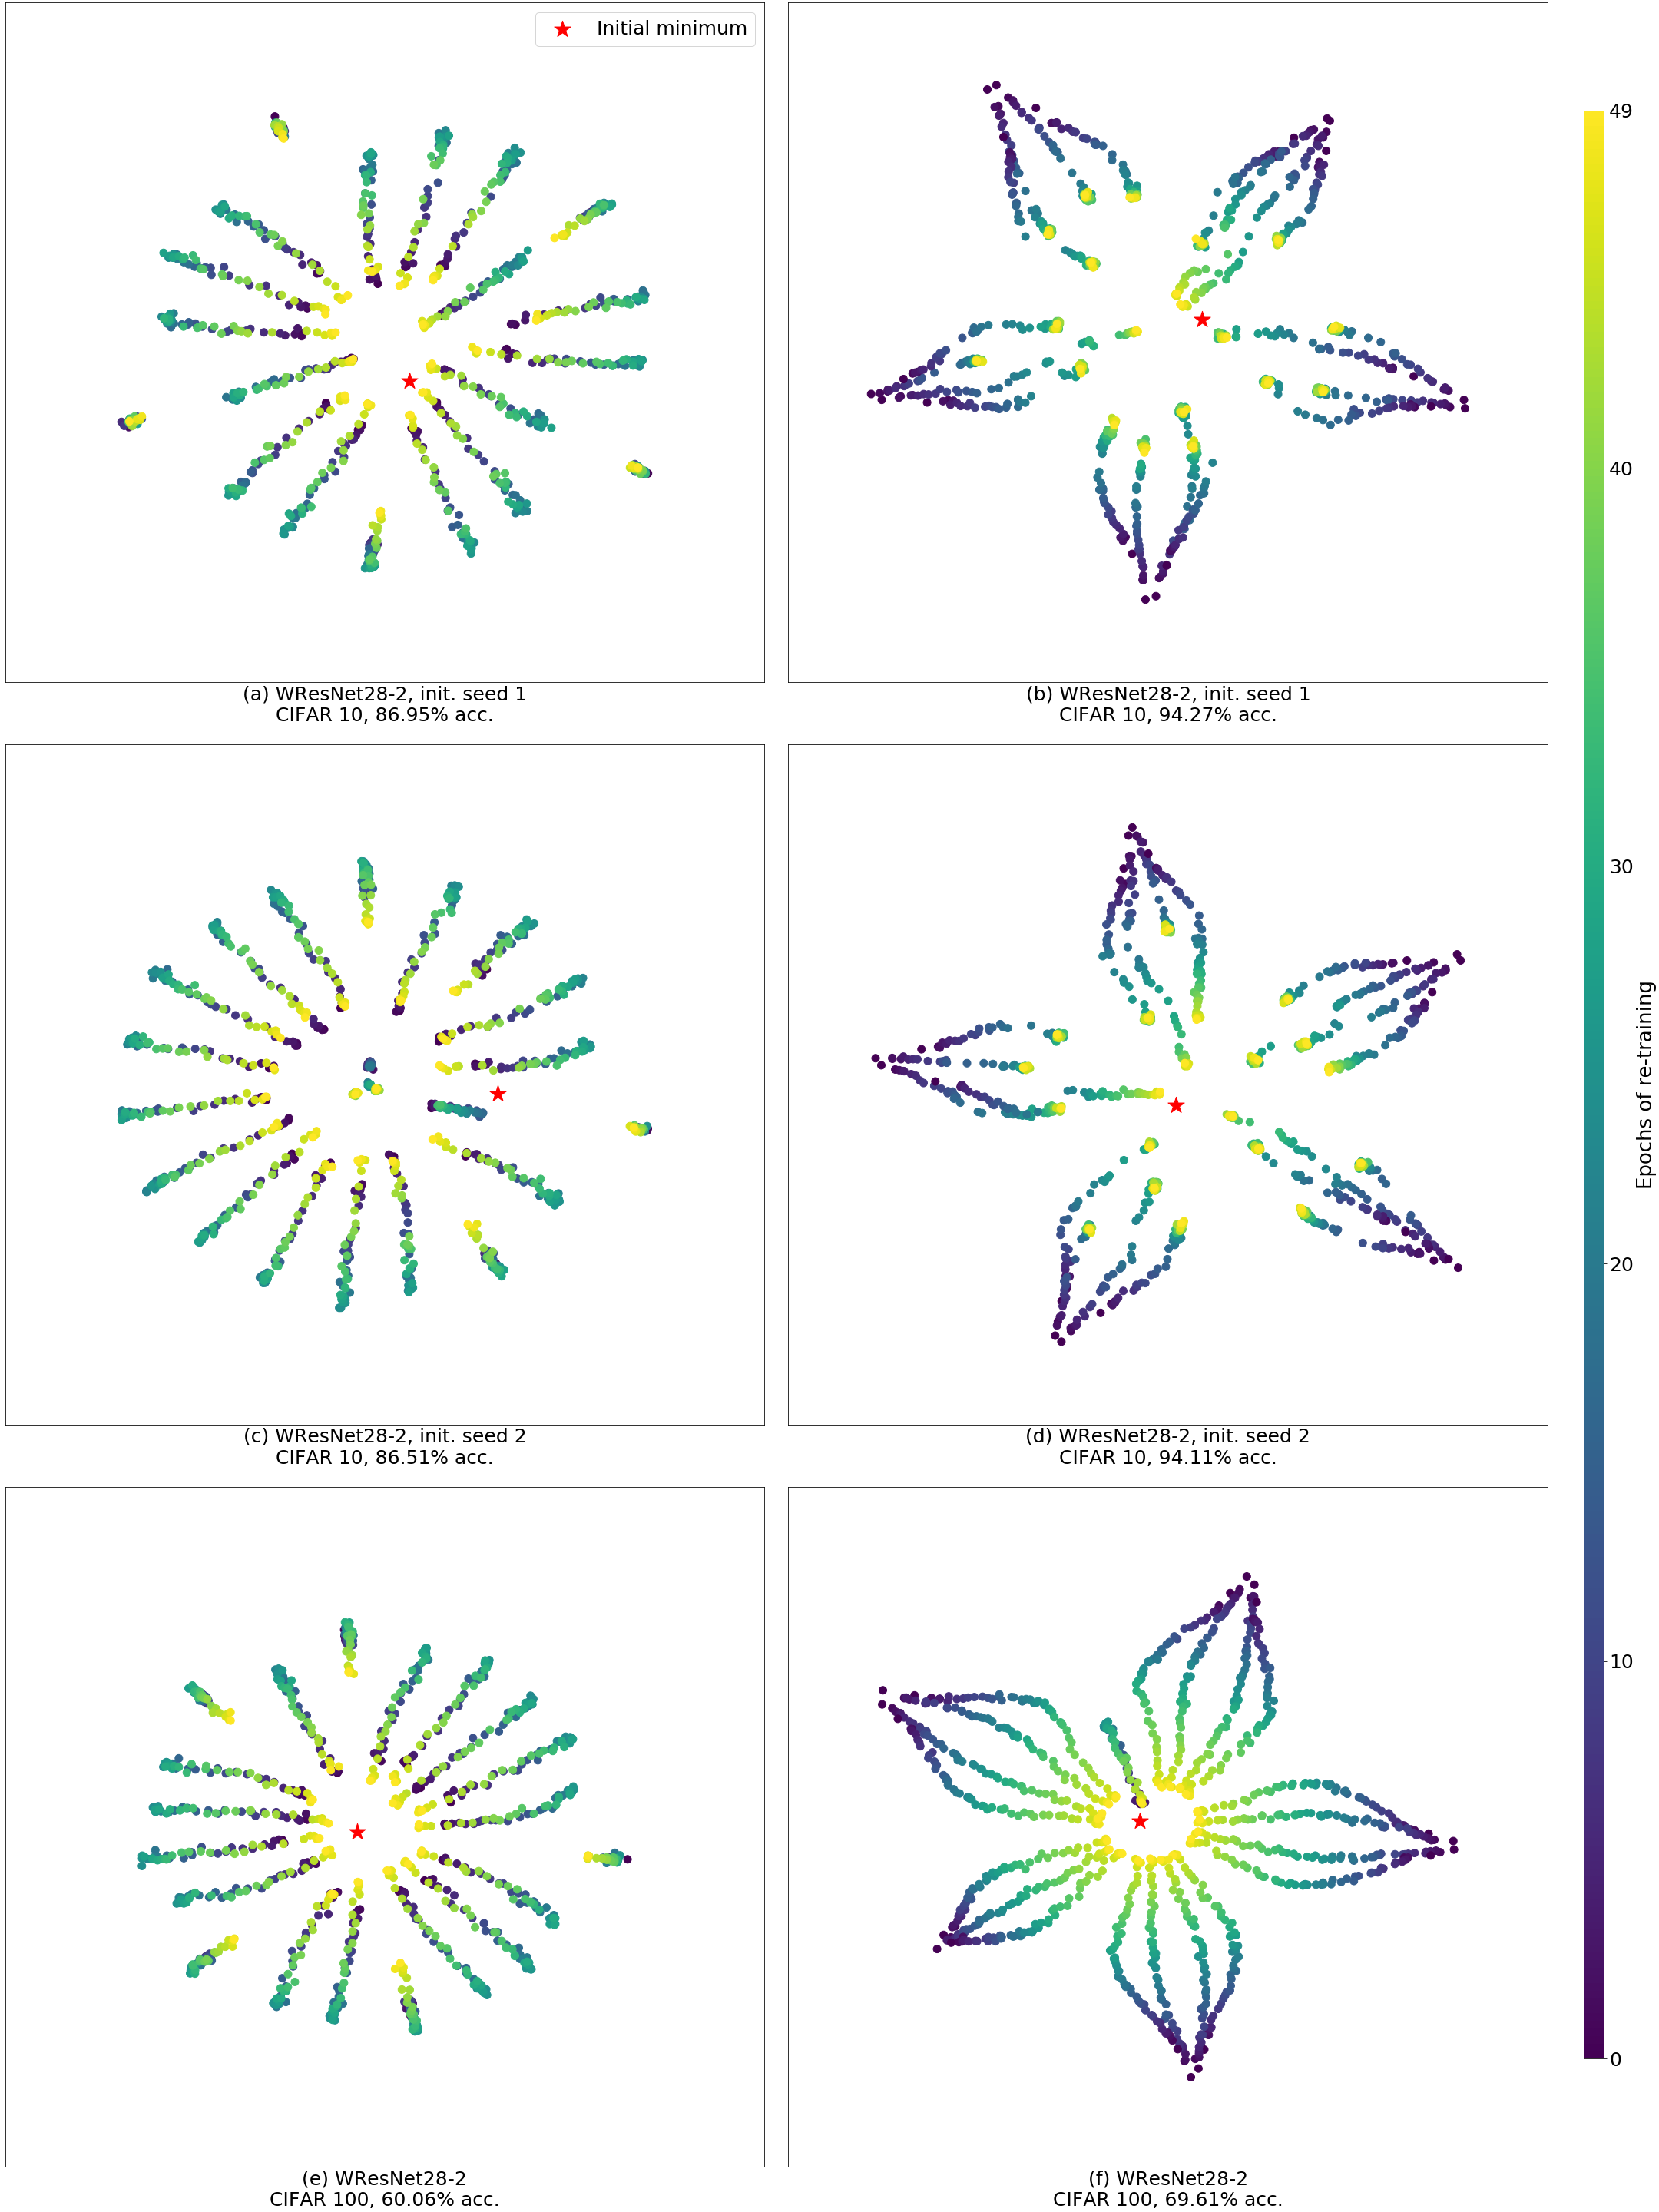}
    \caption{2D PHATE embeddings of the jump and retrain (with 5 random directions here) samples ran on different initialization for the WResNet28-2 network on CIFAR10 (\textbf{a,b,c and d}) and on CIFAR 100 (\textbf{e and f}), colored by epoch of retraining. Patterns that resemble bad generalization are exhibited in the first plot for all three settings as in (a), (c) and (e), while good generalization patterns are shown in the second plots (b), (d) and (f). Since CIFAR100 poses a significantly harder classification task than CIFAR10, our networks only reaches \textasciitilde60\% test accuracy for the bad optimum, and \textasciitilde70\% test accuracy for the good optimum. This is just a reflection of the complexity of the task, with better accuracy requiring a better fine-tuning of the architecture and the training procedure. It demonstrates that our approach is robust across random initializations and tasks.}
    \label{fig:robustness_hi_res}
\end{figure}

\clearpage
\section{}\label{a:additional_examples}
\begin{figure}[H]
    \centering
    \includegraphics[width=0.95\textwidth]{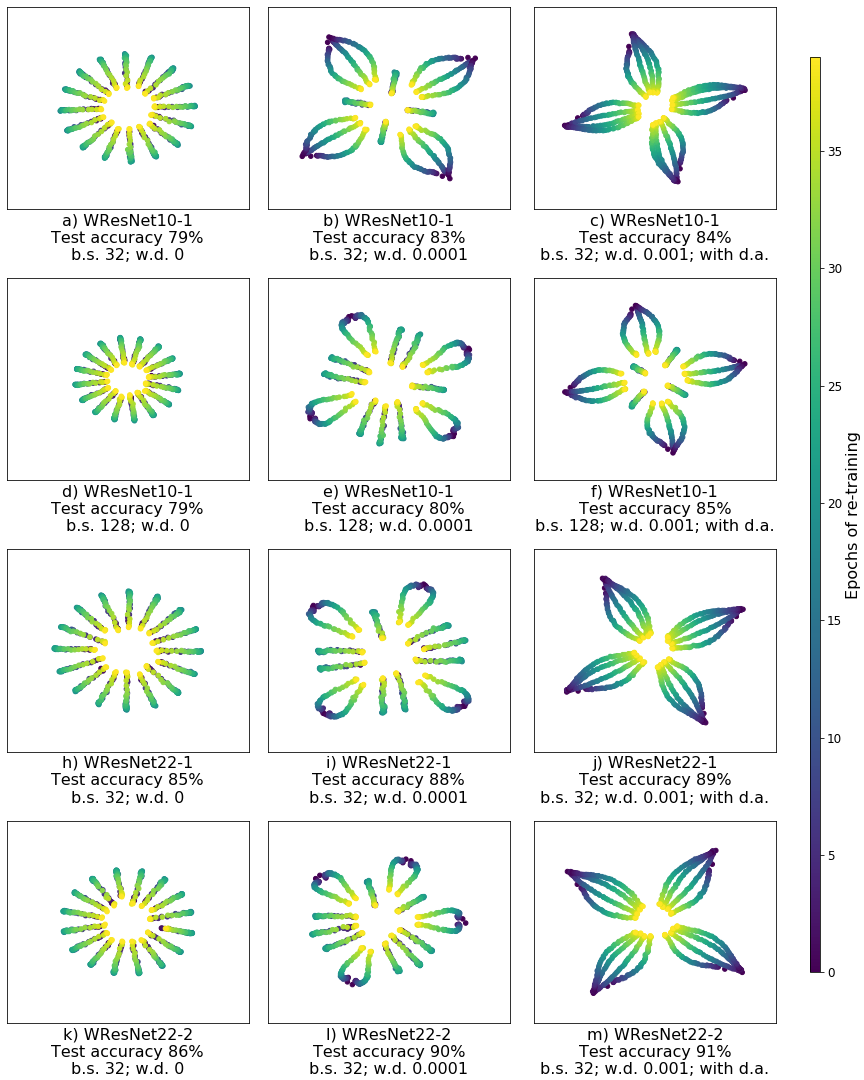}
    \caption{2D PHATE embeddings of the jump and retrain samples ran on different networks, namely a WResNet10-1 trained with a batch size of 32 (a,b,c) and 128 (d,e,f), a WResNet22-1 trained with a batch size of 32 (h,i,j) and a WResNet22-2 trained with a batch size of 32 (k,l,m). The networks in the left column were trained without weight decay and data augmentation. The networks in the middle column were trained with 0.0001 weight decay and no data augmentation. Finally the networks in the right column were trained with 0.001 weight decay and data augmentation. We see that even by keeping network architecture and batch size the same, the regions surrounding optima that generalize better and which were reached with more aggressive forms of regularization seem to have distinct geometrical characteristics which are adequately captured by our sampling and visualization methods.}
    \label{fig:additional_viz_examples}
\end{figure}

% \section{}\label{a:optim_weights_norm}
% \begin{figure}[H]
%     \centering
%     \includegraphics[width=0.95\textwidth]{figures/full_run_weight_L2.png}
%     \caption{L2 norm of network weights during training using different optimizers.}
%     \label{fig:weights norm}
% \end{figure}

% \section{}\label{a:optim_comparison_hi_res}
% \begin{figure}[H]
%     \centering
%     \includegraphics[width=0.95\textwidth]{figures/fig_optimizer_large.pdf}
%     \caption{Higer resolution of Figure~\ref{fig:optim_compare_single}and Figure~\ref{fig:optim_compare_cos}}
%     \label{fig:optim_compare_large}
% \end{figure}
