# Supplementary material for: Exploring the Geometry and Topology of Neural Network Loss Landscapes
Source: arXiv:2102.00485 source file (2022-01-26)
Supplement: Supplementary file 2 [file appendix.tex]

\input{sections/related_work}

\clearpage
\section{}\label{a:dim_red_comparison_hi_res}
\begin{figure}[H]
    \centering
    \includegraphics[width=0.95\textwidth]{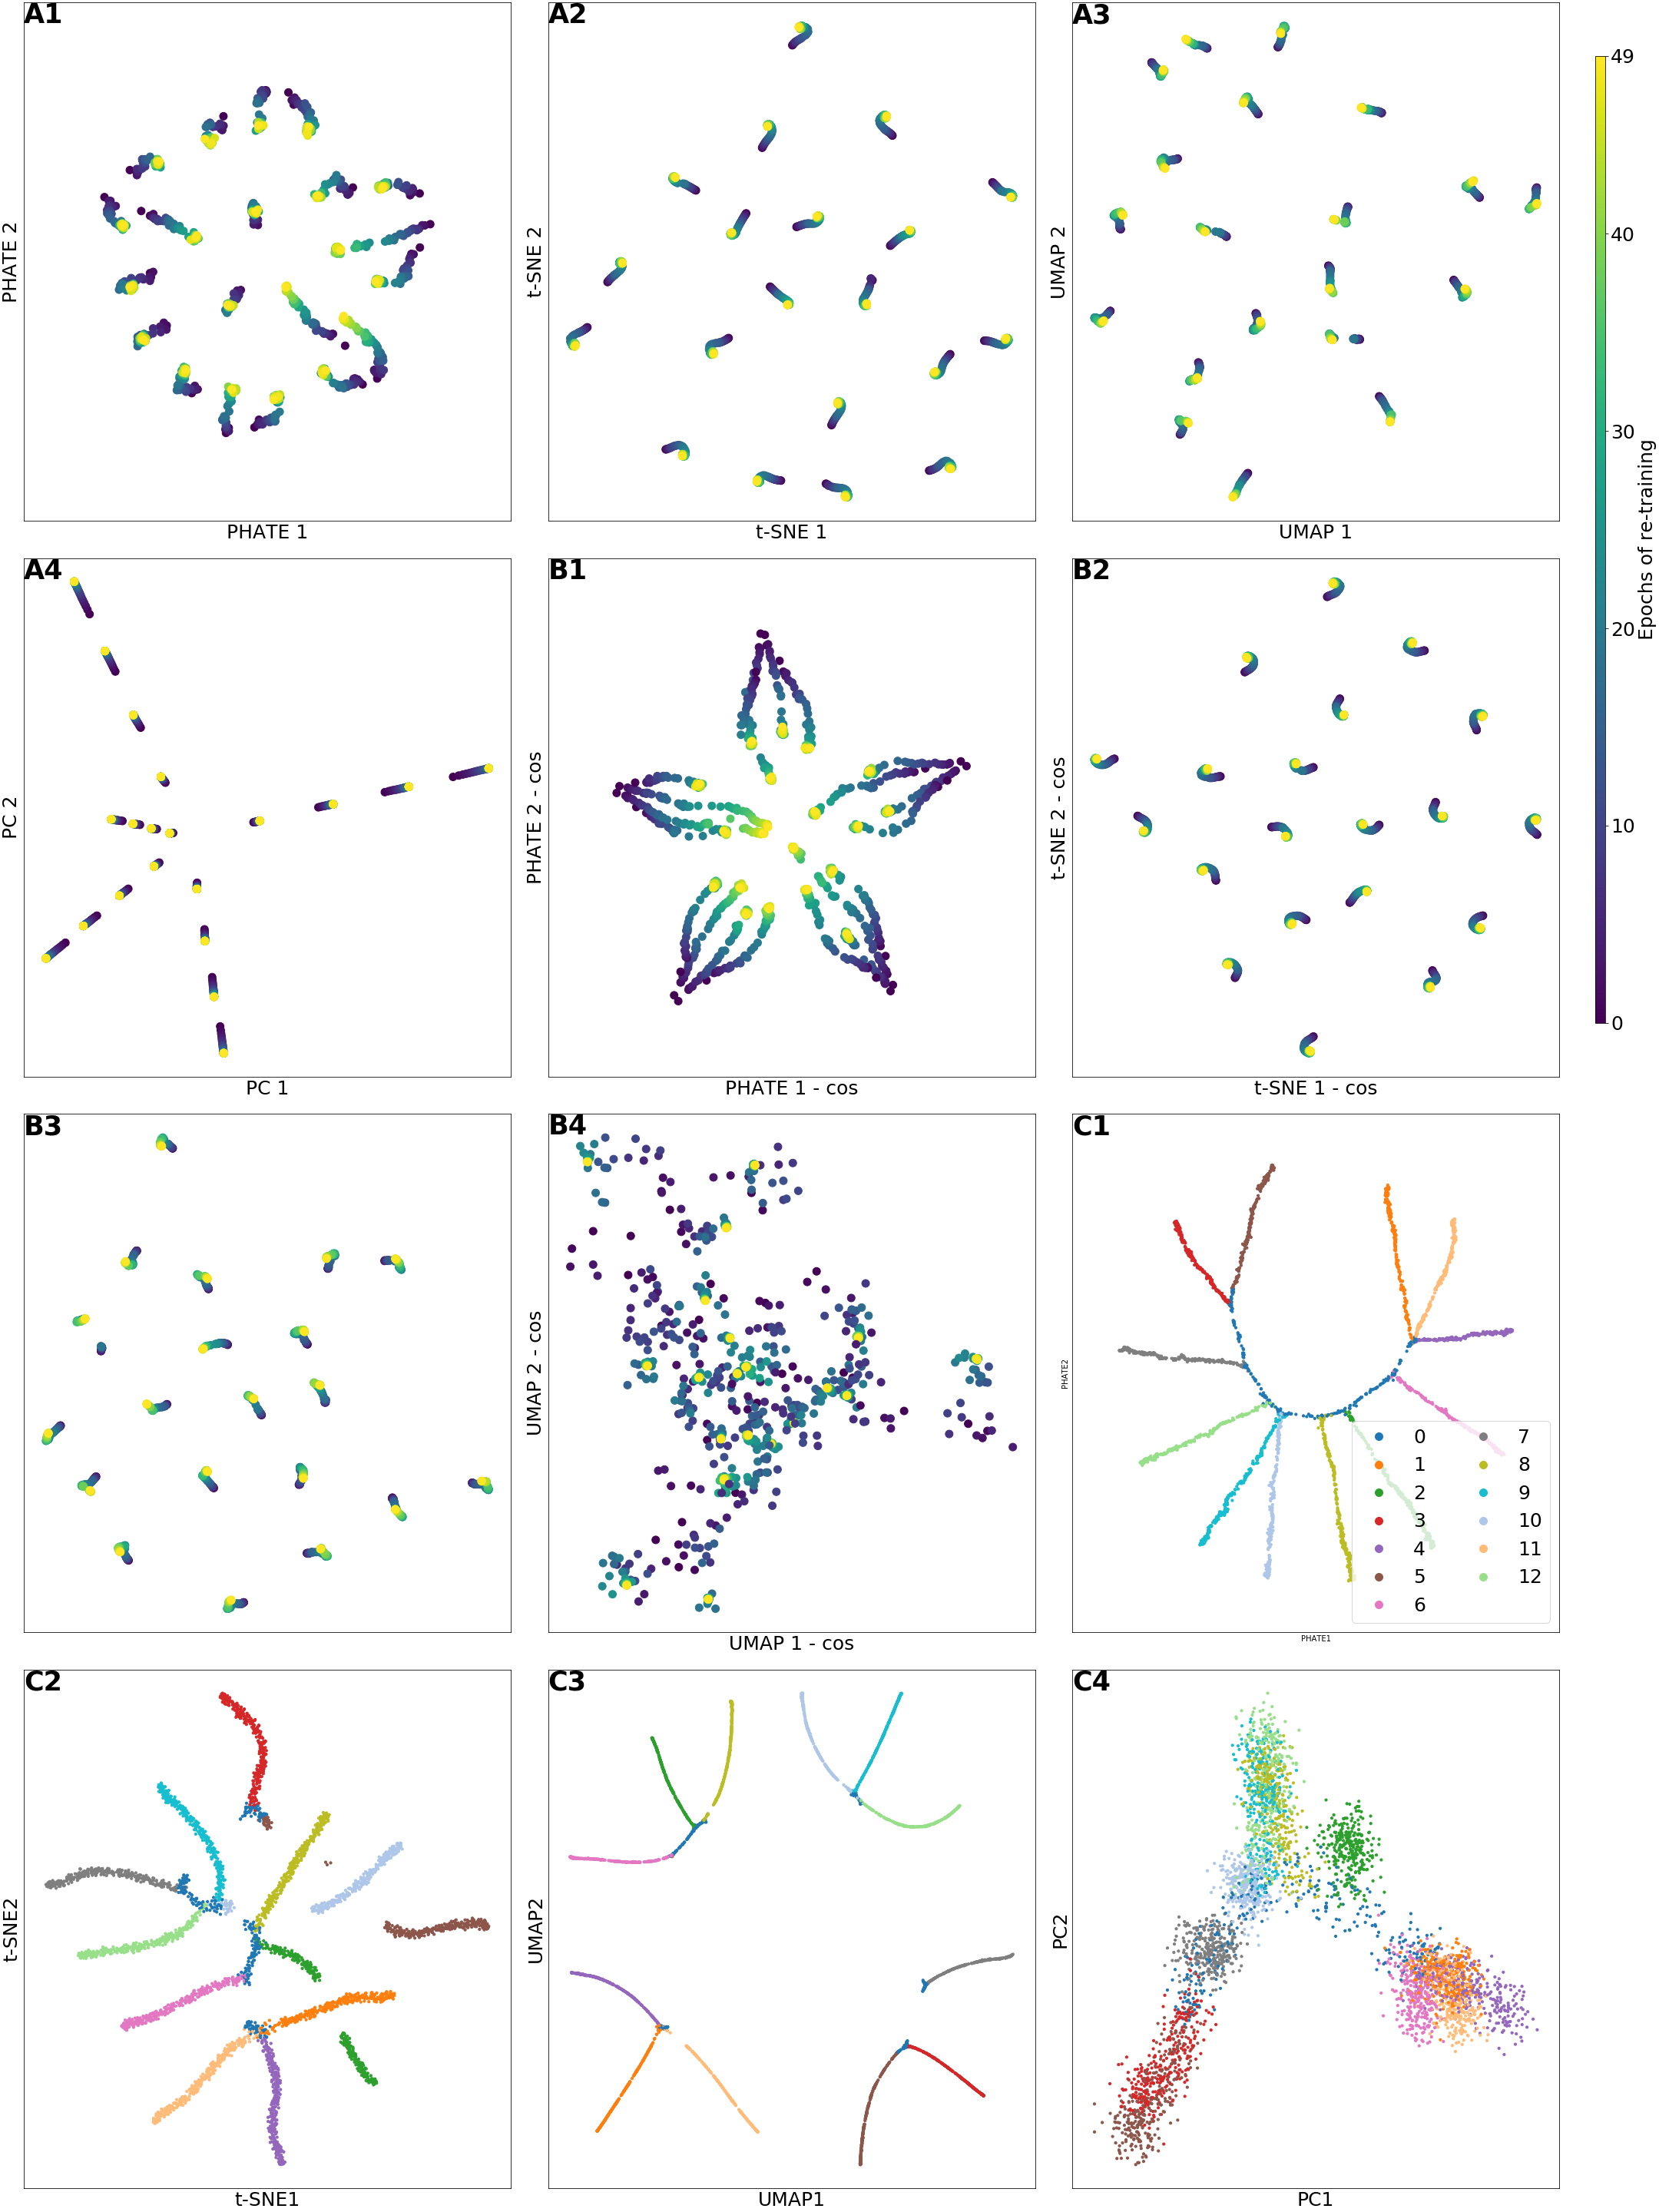}
    \caption{Higher resolutionversion of Figure \ref{fig:dim_red_comparison}}
    \label{fig:dim_red_comparison_hi_res}
\end{figure}

% \section{}\label{a:generalization_hi_res}
% \begin{figure}[H]
%     \centering
%     \includegraphics[width=0.95\textwidth]{figures/generalization_memorization_figure_appendix.png}
%     \caption{Higher resolution version of Figure \ref{fig:generalization}}
%     \label{fig:generalization_hi_res}
% \end{figure}

\clearpage
\section{}\label{a:classifiers}
The 11 classifiers were: k-NN classifier with k=5, linear SVM, RBF kernel SVM, Gaussian Process classifier, decision tree, random forest with 100 trees, MLP classifier with 1 hidden layer of 100 ReLU neurons trained with ADAM, AdaBoost classifier with base classifier a decision tree with depth 1, Gaussian Naive Bayes, Multinomial Naive Bayes and a Quadratic Discriminant Analysis classifier. The classifiers were trained and evaluated using 10-fold cross validation. The Scikit-learn implementations were used for all of them.

\clearpage
\section{}\label{a:robustness_hi_res}
\begin{figure}[H]
    \centering
    \includegraphics[width=0.95\textwidth]{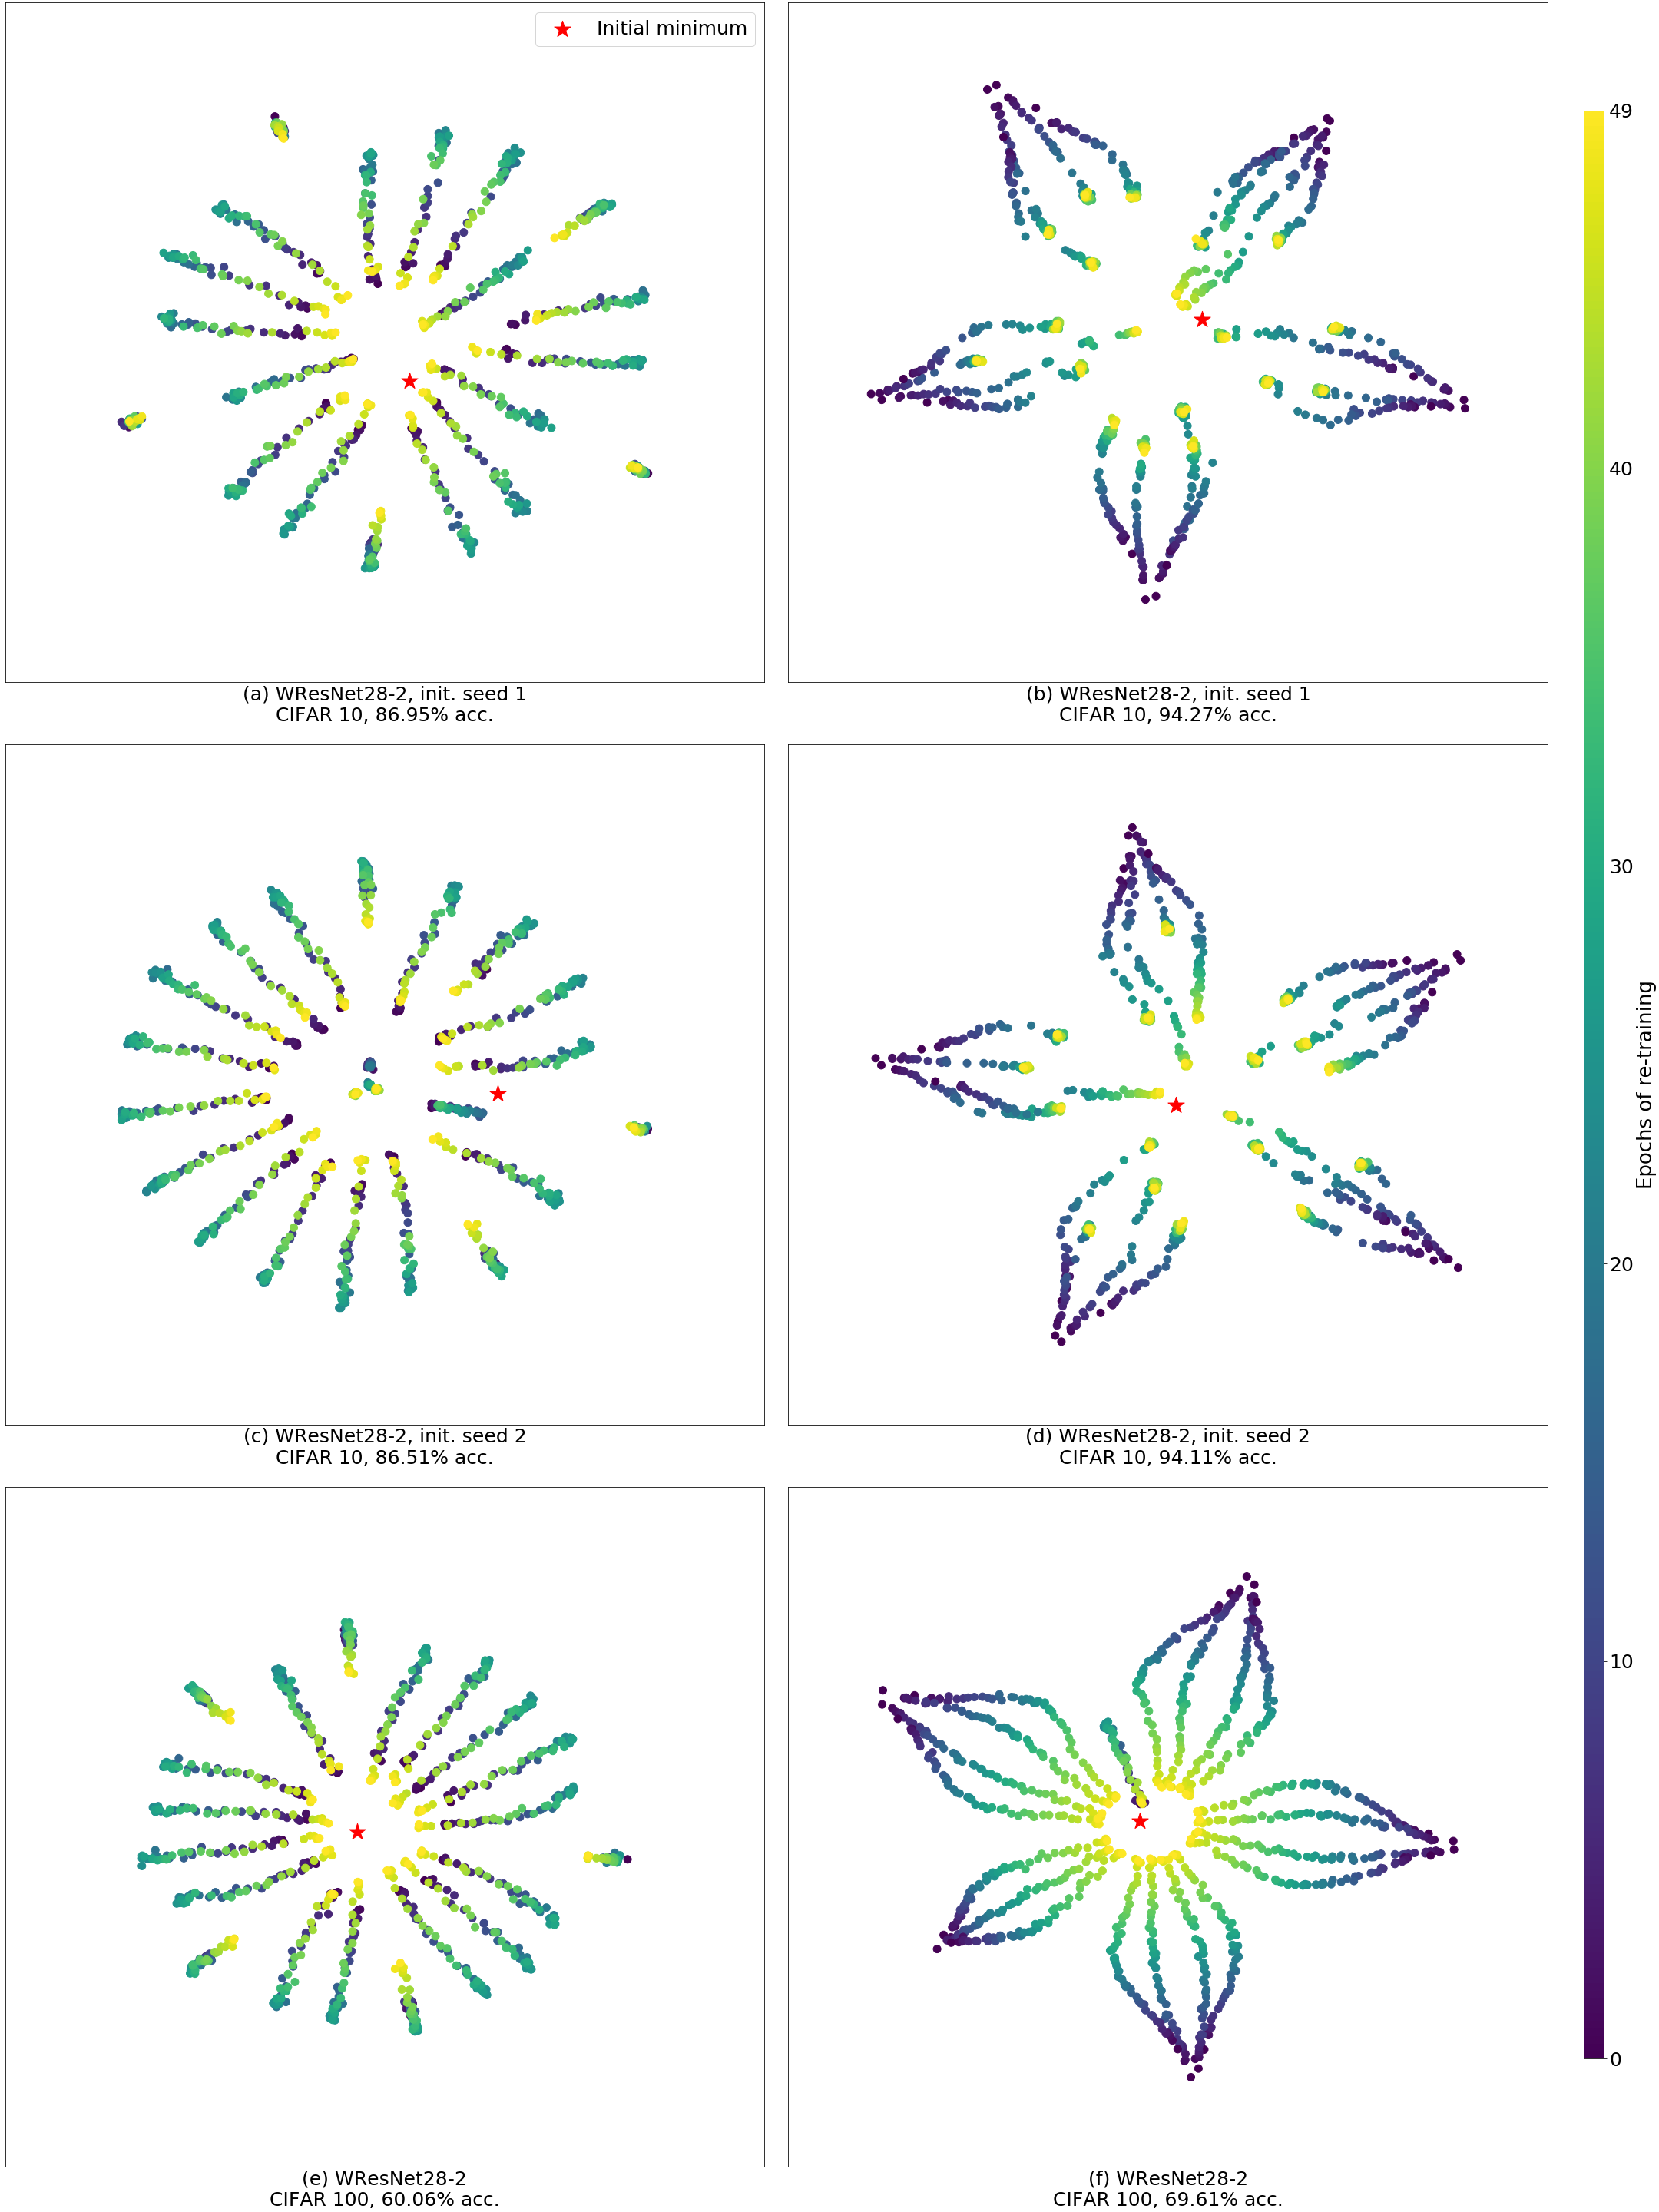}
    \caption{2D PHATE embeddings of the jump and retrain (with 5 random directions here) samples ran on different initialization for the WResNet28-2 network on CIFAR10 (\textbf{a,b,c and d}) and on CIFAR 100 (\textbf{e and f}), colored by epoch of retraining. Patterns that resemble bad generalization are exhibited in the first plot for all three settings as in (a), (c) and (e), while good generalization patterns are shown in the second plots (b), (d) and (f). Since CIFAR100 poses a significantly harder classification task than CIFAR10, our networks only reaches \textasciitilde60\% test accuracy for the bad optimum, and \textasciitilde70\% test accuracy for the good optimum. This is just a reflection of the complexity of the task, with better accuracy requiring a better fine-tuning of the architecture and the training procedure. It demonstrates that our approach is robust across random initializations and tasks.}
    \label{fig:robustness_hi_res}
\end{figure}

\clearpage
\section{}\label{a:additional_examples}
\begin{figure}[H]
    \centering
    \includegraphics[width=0.95\textwidth]{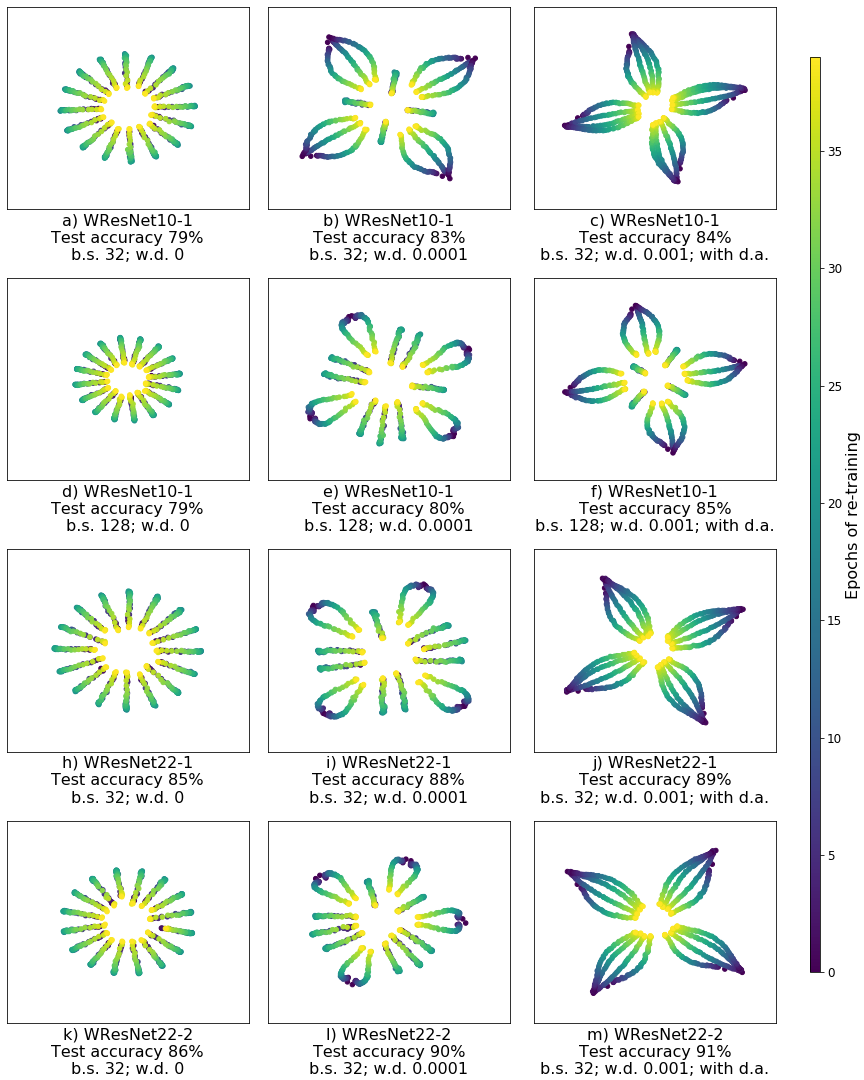}
    \caption{2D PHATE embeddings of the jump and retrain samples ran on different networks, namely a WResNet10-1 trained with a batch size of 32 (a,b,c) and 128 (d,e,f), a WResNet22-1 trained with a batch size of 32 (h,i,j) and a WResNet22-2 trained with a batch size of 32 (k,l,m). The networks in the left column were trained without weight decay and data augmentation. The networks in the middle column were trained with 0.0001 weight decay and no data augmentation. Finally the networks in the right column were trained with 0.001 weight decay and data augmentation. We see that even by keeping network architecture and batch size the same, the regions surrounding optima that generalize better and which were reached with more aggressive forms of regularization seem to have distinct geometrical characteristics which are adequately captured by our sampling and visualization methods.}
    \label{fig:additional_viz_examples}
\end{figure}


% \section{}\label{a:optim_weights_norm}
% \begin{figure}[H]
%     \centering
%     \includegraphics[width=0.95\textwidth]{figures/full_run_weight_L2.png}
%     \caption{L2 norm of network weights during training using different optimizers.}
%     \label{fig:weights norm}
% \end{figure}

% \section{}\label{a:optim_comparison_hi_res}
% \begin{figure}[H]
%     \centering
%     \includegraphics[width=0.95\textwidth]{figures/fig_optimizer_large.pdf}
%     \caption{Higer resolution of Figure~\ref{fig:optim_compare_single}and Figure~\ref{fig:optim_compare_cos}}
%     \label{fig:optim_compare_large}
% \end{figure}
